# Supplementary material for: Ripple edge engineering of graphene nanoribbons
Source: arXiv:1107.1977 source file (2011-10-24)
Supplement: Supplementary file 1 [file sup_mat_paper.pdf]

# Supplementary materials: Ripple edge engineering of graphene nanoribbons

Philipp Wagner,[1,*] Christopher P. Ewels,[1,†] Viktoria V. Ivanovskaya,[1]
Patrick R. Briddon,[2] Amand Pateau,[1] and Bernard Humbert[1]

[1]*Institut des Matériaux Jean Rouxel (IMN), Université de Nantes, CNRS UMR 6502, 44322 Nantes, France*
[2]*School of Electrical, Electronic and Computer Engineering, University of Newcastle, Newcastle upon Tyne, NE 1 7RU, United Kingdom*

| Figure | Graph | a | b | c | standard deviation |
|---|---|---|---|---|---|
| Fig.3,b (Strain) | A (OH-flat) | 48.154 | −46.023 | −0.0480 | 0.050 |
| | B (OH-flat) | 33.149 | −27.726 | 0.137 | 0.036 |
| | C (OH-rippled) | 5.760 | 18.369 | 0.004 | 0.048 |
| | H-terminated (flat) | 3.759 | 3.398 | −0.018 | 0.031 |
| Fig.6,b (Young's Modulus) | C (OH-rippled) | −3.381 | 4.354 | 1.031 | 0.004 |
| | H-terminated (flat) | −1.257 | 0.334 | 1.046 | 0.010 |

TABLE I. Fit parameters of function $y(x) = \frac{a}{x} + \frac{b}{x^2} + c$ when fitting to the curves of strain vs ribbon width Fig.3,b, and Young's Modulus vs ribbon width, Fig.6,b. The fits show that for infinite ribbon widths both the H- and -OH rippled ribbons tend to the same calculated Young's Modulus of about $1.04 \pm 0.01$ TPa. The non-zero coefficient for b indicates non-linear effects that become important for very small ribbon widths.

## I. FORMATION ENERGY OF -OH TERMINATED AGNRS

In Fig.1,a the formation energy $\Delta U_f$:

$$\Delta U_f = (U(GNR) - N_C \cdot U(C_{Graphene}) - 2 \cdot U(H_2) - 2 \cdot U(O_2))/N_{total}$$

is plotted versus armchair graphene nanoribbon (AGNR) width. Here $N_C$ is the number of carbon atoms and $N_{total}$ is the total number of atoms in a fundamental unit cell of length $a_0$. A big energy difference to the flat OH-terminated configuration can be seen. In total the OH-functionalised ANGRs with rippled edges are $\approx$ 0.3 eV/atom more stable than H-terminated flat AGNRs with an $O_2$ reservoir. This shows the strong stability of hydroxyl groups and strengthens the probability to find these groups in experiments. In Fig.1,b only the Young's Modulus for structure B is shown additionally to Figure 4,a in the article.

## II. ESTIMATED ENERGY BARRIER FOR DYNAMIC RIPPLING

We have examined whether the static ripples will dynamically fluctuate at room temperature by calculating the barrier to invert the ripple, however this shows a high barrier and suggests there will not be strong phonon coupling with these ripples. The static character of the rippled edges is demonstrated in Fig.2 where we strain an OH-terminated rippled AGNR. Even straining the AGNR up to 5.5 % the ripples do not flip spontaneously to a flat structure (in the article labelled as Structure B, OH-flat). A nudged elastic band (NEB) calculation[1] was then performed to determine the barrier when strained to the same value as the flat configuration. No barrier was found between the rippled and flat structures, demonstrating that configuration B is a metastable maximum. These two calculations can be summed to estimate the ripple inversion barrier, as demonstated in Fig.2, giving a minimum barrier of $\Delta U_{Barrier} = 0.59$ $eV/a_0$ to invert one edge wave. This barrier is too high for thermal activation at room temperature.

## III. FUNCTIONALISATION OF GRAPHENE NANORIBBONS WITH DIFFERENT GROUPS

We studied a range of other edge functional groups besides hydroxylation such as -F, -Cl and -SH, all of which showed the same edge rippling effect. As complementary example the resultant edge rippling for -F is shown in Fig.3.

* philipp.wagner@cnrs-imn.fr
† chris.ewels@cnrs-imn.fr
[1] G. Henkelman, B. Uberuaga, and H. Jonsson, J. Chem. Phys., **113**, 9901 (2000)

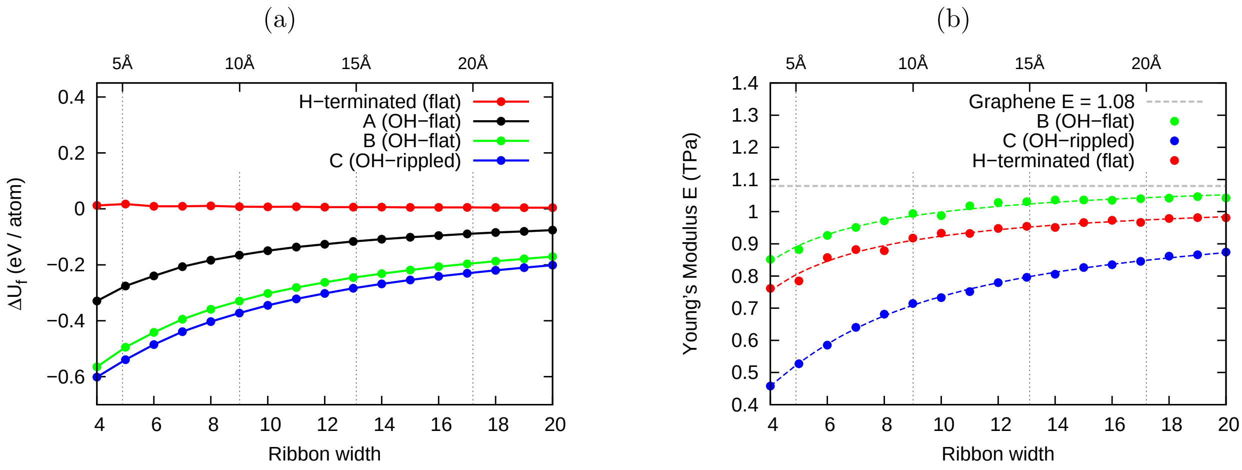


FIG. 1. (a) Formation energy ($\Delta U_f$) for all different structures of -OH terminated functional edges, as a function of ribbon width. (b) Metastable structure B added to the Fig.6,b in the article, showing the Young's Modulus versus width of the AGNRs.

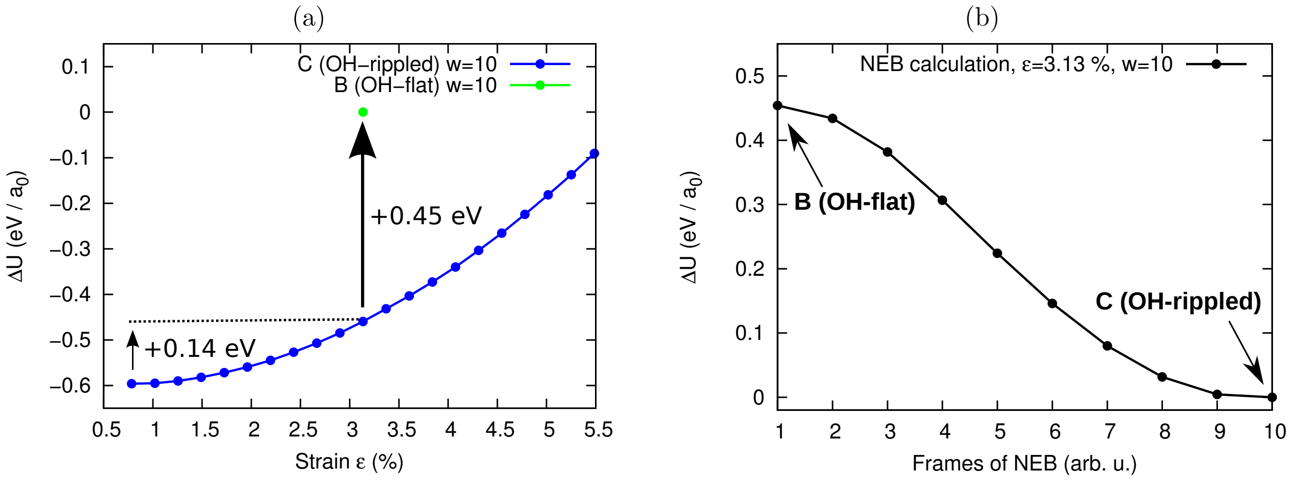


FIG. 2. (a) Estimated energy barrier for dynamic rippling for width 10 with $\Delta U_{Barrier} = 0.14 + 0.45 = 0.59$ eV/$a_0$. (b) No energy barrier is found (NEB-method) between hydroxyl AGNR configurations B and C with same strain ($\epsilon = 3.13$ %), showing configuration B is a metastable maximum.

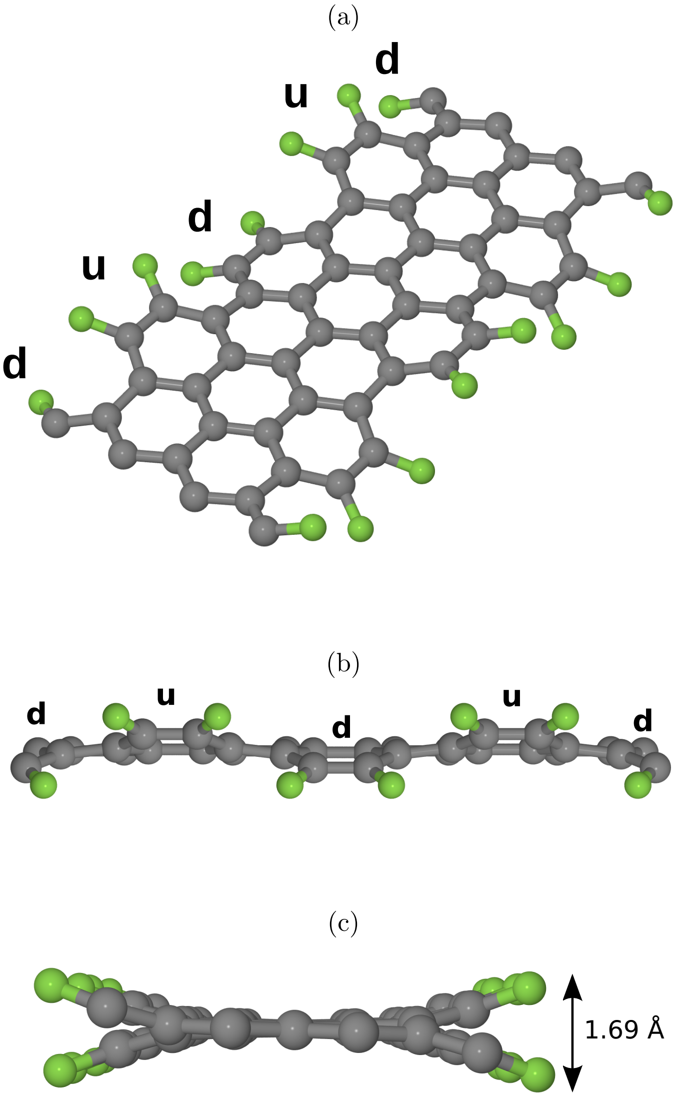


FIG. 3. Armchair graphene nanoribbon (width 7), F-terminated. (a) perspective view, (b) side view, (c) front view. In grey C atoms are pictured, F atoms are green. *u* stands for “up” and *d* for “down” for the rippled edge.
